# Supplementary material for: Joint Manifold Learning and Density Estimation Using Normalizing Flows
Source: arXiv:2206.03293 source file (2022-06-07)
Supplement: Supplementary file 2 [file scores_appendix.tex]

\begin{tabular}{lcccc}
		\toprule
		
		criterion
		& \makecell{PR-D \\ ($3072 \rightarrow 1000$)}
		& \makecell{DNF \\ ($3072 \rightarrow 1000 \rightarrow 1000$)}
		& \makecell{DNF \\ ($3072 \rightarrow 700 \rightarrow 700$)}
		& \makecell{DNF \\ ($3072 \rightarrow 500 \rightarrow 500$)}
		\\
		
		\cmidrule{1-5}\morecmidrules\cmidrule{1-5}
 		FID & 108.71 & 55.45 & ? & 119.50 \\
		MSE & 0.001 $\pm$ 4e-5 & 0.001 $\pm$ 9e-5 & ? & 0.007 $\pm$ 0.0004 \\
		BPD & 4.39 $\pm$ 0.05 & 4.10 $\pm$ 0.04 & ? & 4.25 $\pm$ 0.04 \\
		\#Params & & & & \\

		\bottomrule
\end{tabular}
