# Supplementary material for: Joint Manifold Learning and Density Estimation Using Normalizing Flows
Source: arXiv:2206.03293 source file (2022-06-07)
Supplement: Supplementary file 3 [file scores_appendix3.tex]

\begin{tabular}{lcccc}
		\toprule
		
		criterion
		& \makecell{EE-M \\ {\tiny ($3072 \rightarrow 1000 \rightarrow 500$)}}
		& \makecell{EE-H \\ {\tiny ($3072 \rightarrow 1000 \rightarrow 500$)}}
		& \makecell{H-MM$^\star$ \\ {\tiny ($3072 \rightarrow 1000 \rightarrow 500$)}}
		& \makecell{H-HH$^\star$ \\ {\tiny ($3072 \rightarrow 1000 \rightarrow 500$)}}
		\\
		
		\cmidrule{1-5}\morecmidrules\cmidrule{1-5}
 		FID & & 157.71 & &  \\
		MSE & & 0.001 $\pm$ 3e-5 & &  \\
		BPD & & 4.20 $\pm$ 0.05 & &  \\
% 		\#Params & & & & \\

		\bottomrule
\end{tabular}
